# Supplementary material for: Topological Phases in InAs$_{1-x}$Sb$_x$: From Novel Topological Semimetal to Majorana Wire
Source: arXiv:1602.07001 source file (2016-07-18)
Supplement: Supplementary file 1 [file supplementary_material.pdf]

# Supplementary Material for "Topological Phases in $InAs_xSb_{1-x}$: From Novel Topological Semimetal to Majorana Wire"

Georg W. Winkler[1], QuanSheng Wu[1], Matthias Troyer[1], Peter Krogstrup[2], and Alexey A. Soluyanov[1,3]

[1]Theoretical Physics and Station Q Zurich, ETH Zurich, 8093 Zurich, Switzerland
[2]Center for Quantum Devices and Station Q Copenhagen, Niels Bohr Institute, University of Copenhagen, 2100 Copenhagen, Denmark
[3]Department of Physics, St. Petersburg State University, St. Petersburg, 199034 Russia

Here we provide details on (additional) first principles calculations, tight-binding models, derivation of $\mathbf{k}\cdot\mathbf{p}$ models, details on the topological classification and Landé $g$-factor calculation.

## 1 First-principles simulations

The first-principles calculations were performed in the Vienna *ab initio* simulation package (VASP) [1, 2] with the projector augmented-wave method, using a cut-off energy of 300 eV. The Brillouin zone (BZ) integration was done with Monkhorst-Pack meshes. We used 8×8×8 for pure InAs/InSb, 6×6×6 for CuPt-ordered $InAs_{0.5}Sb_{0.5}$, 6×6×2 for 2-layer $InAs_{0.67}Sb_{0.33}/InAs_{0.33}Sb_{0.67}$ and a 4×4×4 $k$-point mesh for the 8 atoms supercells. The later calculation was used for testing the ETB models. The lattice constants for pure InAs and InSb were taken from the work of Ref. [3]. We used VASP pseudopotentials generated with the generalized gradient approximation for the exchange-correlation potential as implemented by Perdew–Burke–Ernzerhof [4]. The HSE06 hybrid functional was employed for all first-principles calculations [5, 6, 7].

During the relaxation the cut-off energy was increased to 380 eV. The relaxed structure for CuPt-ordered $InAs_{0.5}Sb_{0.5}$ is given in Tab. 1. The primitive lattice can be embedded in a nearly cubic superlattice as illustrated in Fig. 1. There the sum $\mathbf{a}_1 + \mathbf{a}_2 + \mathbf{a}_3$ gives the vertical edge of the cube. Since the $x$ and $y$-component of $\mathbf{a}_1 + \mathbf{a}_2 + \mathbf{a}_3$ are nonzero the cube is slightly distorted. The 001 and 111 strains were applied such that the volume of the unit cell is preserved.

The total energy per atom of the resulting structure is -4.4432 eV which is in between the energies of pure InAs -4.6458 eV and InSb -4.2900 eV. This hints, together with the experimental evidence [8], at the stability of this ordering.

| | $x$ [Å] | $y$ [Å] | $z$ [Å] | | $a_1$ | $a_2$ | $a_3$ |
|---|---|---|---|---|---|---|---|
| $a_1$ | -3.1584 | 0.0000 | 3.1584 | In | -0.0047 | -0.0047 | 0.0140 |
| $a_2$ | 0.0000 | -3.1584 | 3.1584 | In | 0.5045 | 0.5045 | 0.4865 |
| $a_3$ | 3.1617 | 3.1617 | 6.3200 | As | 0.8747 | 0.8747 | 0.3758 |
| | | | | Sb | 0.3755 | 0.3755 | 0.8736 |

Table 1: Lattice vectors and atomic positions in reduced coordinates for the fully relaxed CuPt-ordered $InAs_{0.5}Sb_{0.5}$.

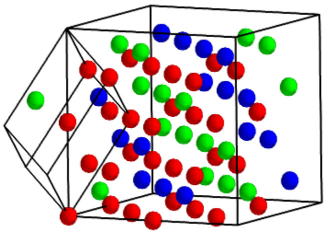

Figure 1: Primitive and cubic unit cells of the CuPt-ordered structure.

| Material | | (111) | (110) | (001) | $(1\bar{1}0)$ | $(11\bar{2})$ |
|---|---|---|---|---|---|---|
| $Al_{0.5}Ga_{0.5}As$ | $\alpha$ [eV Å] | 0.0 | 0.08 | 0.11 | 0.13 | 0.13 |
| | $E_{\mathrm{SO}}$ [meV] | 0.0 | 0.04 | 0.07 | 0.1 | 0.1 |
| | $m^*$ [$m_e$] | 0.34 | 0.28 | 0.24 | 0.21 | 0.21 |
| | $l_{\mathrm{R}}$ [Å] | $\infty$ | 360 | 290 | 270 | 270 |
| | $E_g$ [$K$] | 0.0 | 0.01 | 0.02 | 0.03 | 0.03 |
| $Al_{0.5}In_{0.5}As$ | $\alpha$ [eV Å] | 0.0 | 0.07 | 0.09 | 0.11 | 0.11 |
| | $E_{\mathrm{SO}}$ [meV] | 0.0 | 0.02 | 0.04 | 0.06 | 0.06 |
| | $m^*$ [$m_e$] | 0.24 | 0.21 | 0.18 | 0.17 | 0.17 |
| | $l_{\mathrm{R}}$ [Å] | $\infty$ | 660 | 440 | 400 | 400 |
| | $E_g$ [$K$] | 0.0 | 0.002 | 0.006 | 0.01 | 0.01 |

Table 2: Linear spin splitting coefficient $\alpha$ and $E_{\mathrm{SO}}$ for different $k$-space directions for the CuPt-ordered compounds without strain. The spin-orbit precession length $l_{\mathrm{R}} = \hbar^2/m^*\alpha$ is also shown. $E_g$ is calculated using Al as the bulk superconductor and assuming a mobility of $\mu = 10^3\,\mathrm{cm}^2/\mathrm{Vs}$.

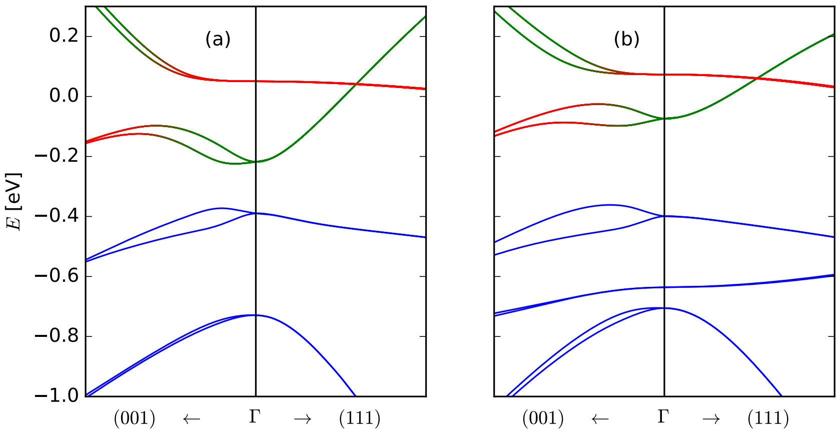


Figure 2: Band structures (HSE06) of the CuPt-ordered $InAs_{0.67}Sb_{0.33}$ (a) and $InAs_{0.33}Sb_{0.67}$ (b).

| | $E(s,a)$ | $E(s,c)$ | $E(p,a)$ | $E(p,c)$ | $E(s^*,a)$ | $E(s^*,c)$ | $V(s,s)$ | $V(x,x)$ |
|---|---|---|---|---|---|---|---|---|
| InAs | -9.6858 | -2.8259 | 0.9577 | 3.7241 | 7.4099 | 6.6101 | -5.8235 | 1.8886 |
| InSb | -7.3190 | -2.8259 | 1.0134 | 3.7241 | 6.9969 | 6.6101 | -5.7081 | 1.2220 |
| | $V(x,y)$ | $V(sa,pc)$ | $V(sc,pa)$ | $V(s^*a,pc)$ | $V(pa,s^*c)$ | $V(s^*,s^*)$ | $\Delta_a$ | $\Delta_c$ |
| InAs | 4.6528 | 4.0628 | 5.0267 | 3.9630 | 3.0000 | 0.0000 | 0.4000 | 0.3920 |
| InSb | 4.0639 | 4.6255 | 4.5736 | 3.0636 | 3.0000 | 0.0000 | 0.8000 | 0.3920 |

Table 3: ETB parameters for InAs and InSb in Slater-Koster notation.

In Tab. 2 we show spin-splitting and related quantities for the CuPt-ordered compounds $Al_{0.5}Ga_{0.5}As$ and $Al_{0.5}In_{0.5}Sb$, which have normal band ordering at zero strain and exhibit the largest values of $E_{SO}$. For the first-principles simulations we used the same parameters as for $InAs_{0.5}Sb_{0.5}$ given above.

We tested the stability of the band inversion in CuPt-ordered $InAs_xSb_{1-x}$ to disorder in the ordering of layers. For $x = 0.33$ (two As-layers and one Sb-layer) and $x = 0.67$ (one As-layer and two Sb-layers), there is still a strong band inversion as shown in Fig. 2.

# 2 Empirical tight-binding calculations for disordered $InAs_xSb_{1-x}$

The parameters for the empirical tight-binding (ETB) models used in the main text are listed in Tab. 3 using the Slater-Koster notation [9]. The parameters were obtained by fitting the ETB band structure to the first-principles band structure. To ensure that the tight-binding parametrizations of InAs and InSb are compatible the In atom was described universally, so that In has the same onsite energies in both InAs and InSb ETBs. Figure 3 shows a good agreement between the ETB bands compared to the first-principles result.

ETB results of small disorder configurations in an 8 atoms cubic supercell were compared versus first-principles calculations, and found to be in good

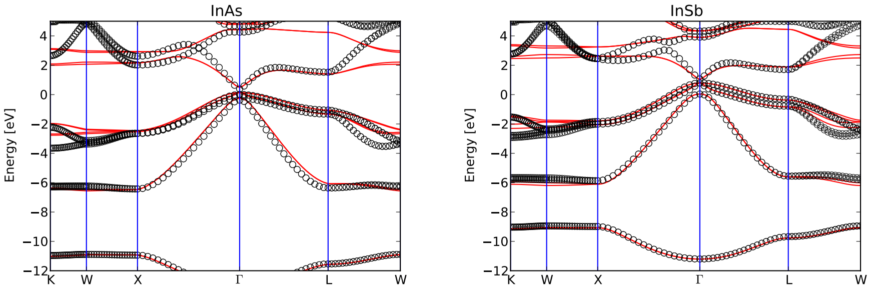


Figure 3: Comparison of ETB (solid red lines) and HSE06 (black open circles) ab initio band structures.

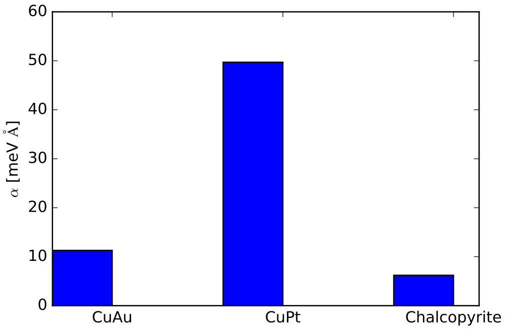


Figure 4: Rashba coefficient $\alpha$ in the (001)-direction of ordered superstructures in $InAs_{0.5}Sb_{0.5}$.

agreement. For the supercell sizes shown in Fig. 1(e-d) of the main text we then used ETB calculations only. For each supercell size 31 Sb concentrations were simulated. Every Sb concentration was averaged between 1000 (for 64 atoms supercell) and 20 (for 1728 atoms supercell) random supercell configurations. The energy gap $E_0$ is plotted for the largest disorder configuration (1728 atoms) and shows negligible dependence on supercell size. The spin-orbit gap $\Delta_0$ is plotted from the 216 atoms supercell, since for larger supercells band folding makes an identification of the correct gap difficult. $\Delta_0$ also shows negligible size dependence between the 8, 64 and 216 atoms supercell. The absolute value of the Rashba coefficient $\alpha$ was extracted from a third order polynomial fit using six data points between $k = 0$ and 0.05 Å in the 110 direction. Then $\alpha$ was averaged over disorder configurations.

Apart from the disorder simulations, the ETB models were also used to simulate and analyze different ordered supercells. In Fig. 4 we compare the CuAu-, CuPt- and chalcopyrite-ordering in terms of spin-splitting along the (001) direction. The CuPt-type ordering shows the most promising spin-splitting of these structures.

| | $\sigma_v$ | $C_3$ | TR |
|---|---|---|---|
| action on $\mathbf{k}$ | $\begin{pmatrix} 1 & & \\ & -1 & \\ & & 1 \end{pmatrix}$ | $\begin{pmatrix} -\frac{1}{2} & -\frac{\sqrt{3}}{2} & \\ \frac{\sqrt{3}}{2} & -\frac{1}{2} & \\ & & 1 \end{pmatrix}$ | $\begin{pmatrix} -1 & & \\ & -1 & \\ & & -1 \end{pmatrix}$ |
| representation $R$ | $\begin{pmatrix} -i & & & \\ & i & & \\ & & i & \\ & & & -i \end{pmatrix}$ | $\begin{pmatrix} -1 & & & \\ & -1 & & \\ & & \frac{1}{2} & -\frac{\sqrt{3}}{2} \\ & & \frac{\sqrt{3}}{2} & \frac{1}{2} \end{pmatrix}$ | $\begin{pmatrix} 0 & \frac{1-i}{\sqrt{2}} & & \\ \frac{-1+i}{\sqrt{2}} & 0 & & \\ & & 0 & -1 \\ & & 1 & 0 \end{pmatrix}\mathcal{K}$ |

Table 4: Symmetries and representations of the $C_{3v}$ double group. $\mathcal{K}$ is the complex conjugation operator.

# 3 $\mathbf{k}\cdot\mathbf{p}$ models

A $\mathbf{k}\cdot\mathbf{p}$ description of the crossing point is obtained from group theoretical considerations. First, the representations of the symmetries need to be found. The point group at the crossing point is $C_{3v}$, therefore we need to consider the $C_3$ and $\sigma_v$ symmetries. In the following we assume $z$ to be the threefold rotation axis and $xz$ to be the mirror plane. In Tab. 4 we list the symmetries and their representations. It is easy to check that these representations fulfill the expected relations for spin-$\frac{1}{2}$ particles, e.g. $(C_3)^3 = (\sigma_v)^2 = -\mathbf{1}$ and they commute with the time-reversal (TR) operator.

Let us first construct a $\mathbf{k}\cdot\mathbf{p}$ description around the crossing point at $\mathbf{k}_c = (0, 0, 0.0646)\ [\text{Å}^{-1}]$. The Hamiltonian has to be symmetric under the symmetries of the little group ($\sigma_v$, $C_3$), that is

$$H(\sigma_v \cdot \mathbf{k}) = R_{\sigma_v}\, H(\mathbf{k})\, R^\dagger_{\sigma_v},$$
$$H(C_3 \cdot \mathbf{k}) = R_{C_3}\, H(\mathbf{k})\, R^\dagger_{C_3}.$$

Under the above constrains, to linear order in $\mathbf{k}$, the Hamiltonian is given by

$$H_{\mathbf{k}\cdot\mathbf{p}} = \begin{pmatrix} E_0 + A_1 k_z & 0 & D\ k_y & D\ k_x \\ 0 & -E_0 + A_2 k_z & F^* k_x & -F^* k_y \\ D^* k_y & F\ k_x & Bk_z + Ck_x & C\ k_y \\ D^* k_x & -F\ k_y & C\ k_y & Bk_z - Ck_x \end{pmatrix}. \quad (1)$$

In the main text it was assumend that $A_1 = A_2$, which is not dictated by symmetry but almost perfectly fulfilled in the case of CuPt-ordered $InAs_{0.5}Sb_{0.5}$. In Fig. 3(b) of the main text we break the $\sigma_v$ symmetry via adding a local term of the form

$$\gamma \begin{pmatrix} 0 & 1 & & \\ 1 & 0 & & \\ & & 0 & -i \\ & & i & 0 \end{pmatrix}, \quad (2)$$

where we used $\gamma = 0.0005$.

Analogously, a $\mathbf{k}\cdot\mathbf{p}$ model around the zone center $\Gamma$ can be constructed. In this case the TR symmetry is also included in the little group. Up to quadratic order in $\mathbf{k}$, the Hamiltonian is given by

$$H^\Gamma_{\mathbf{k}\cdot\mathbf{p}} = \begin{pmatrix} \epsilon_1(\mathbf{k}) + A_1 k_z & 0 & \omega B k_y & \omega B k_x \\ 0 & \epsilon_1(\mathbf{k}) - A_1 k_z & -B^* k_x & B^* k_y \\ \omega^* B^* k_y & -B k_x & \epsilon_2(\mathbf{k}) + A_2 k_x & A_2 k_y \\ \omega^* B^* k_x & B k_y & A_2 k_y & \epsilon_2(\mathbf{k}) - A_2 k_x \end{pmatrix}, \quad (3)$$

| $E_0$(eV) | $A_1$(eV Å) | $A_2$(eV Å) | $B$(eV Å) | $C$(eV Å) | $D$(eV Å) | $E$(eV Å) | $F$(eV Å) |
|---|---|---|---|---|---|---|---|
| 0.1696 | 0.02 | 1.26 | 1.48 | -5.86 | 14.3 | -3.91 | 54.2 |

Table 5: Parameters of the fitted $\mathbf{k}\cdot\mathbf{p}$ model around $\Gamma$.

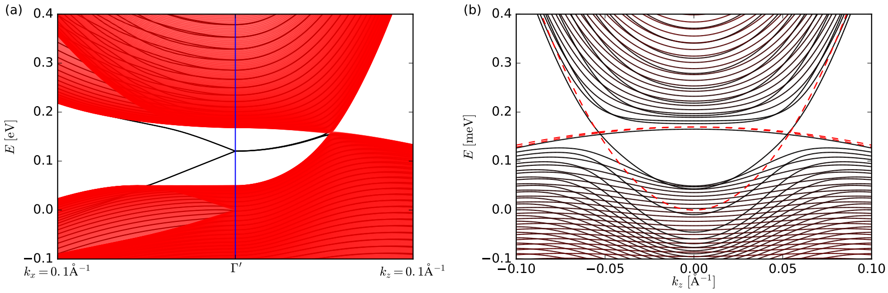

Figure 5: (a) The surface states of the $\mathbf{k}\cdot\mathbf{p}$-model given in Eq. (3) in a slab geometry terminated in a $xz$-surface. (b) Landau level calculation for a magnetic field of 50 Tesla in the $z$-direction. The red dashed line is the original band structure of the $\mathbf{k}\cdot\mathbf{p}$-model.

with $\omega = \frac{1-i}{\sqrt{2}}$ and

$$\epsilon_1 = E_0 + C(k_x^2 + k_y^2) + Ek_z^2$$
$$\epsilon_2 = D(k_x^2 + k_y^2) + Fk_z^2.$$

If $A_1$ and $A_2$ are set to zero inversion symmetry is restored and the model describes a Dirac semimetal. In Tab. 5 we give a set of parameters fitted to our HSE06 first-principles calculations of $InAs_{0.5}Sb_{0.5}$. By discretizing $k_y$ (see e.g. Ref. [10]) we calculated the surface states on the $xz$-surface in a slab geometry in Fig. 5(a). The qualitative behaviour of the surface states agrees with Fig. 4(a) of the main text. Furthermore, we calculate the Landau level spectrum for a magnetic field of 50 Tesla applied in the $z$-direction in Fig. 5(b). We do this by performing a Peierls substitution, replacing $k_x$ and $k_y$ in Eq. (3) by the corresponding operators in the presence of magnetic fields (see e.g. Ref. [11] for details). We find two gapless Landau levels crossing, similar to the case of a Dirac semimetal [11].

# 4 Evaluation of the chiral charge

The evaluation of the chiral charge, leading to the results shown in Fig. 3(b) of the main text, is faciliated by measuring the Berry flux through a closed surface containing the semimetallic point(s). We choose the surface to be a sphere, on which the Hamiltonian is gapped. Then the topology of this surface is characterized by a Chern number [12], or can also be characterized by a $\mathbb{Z}_2$ quantum number if additional symmetries are present [13]. We evaluate the topology by tracking the hybrid Wannier charge centers (see Ref. [14] for further details) using the software package Z2Pack [15].

In Fig. 6 we present the results obained using the $\mathbf{k}\cdot\mathbf{p}$-model of Eq. (1) with $\sigma_v$ breaking term of the form in Eq. (2) added. In Fig. 6(a) we show the Chern

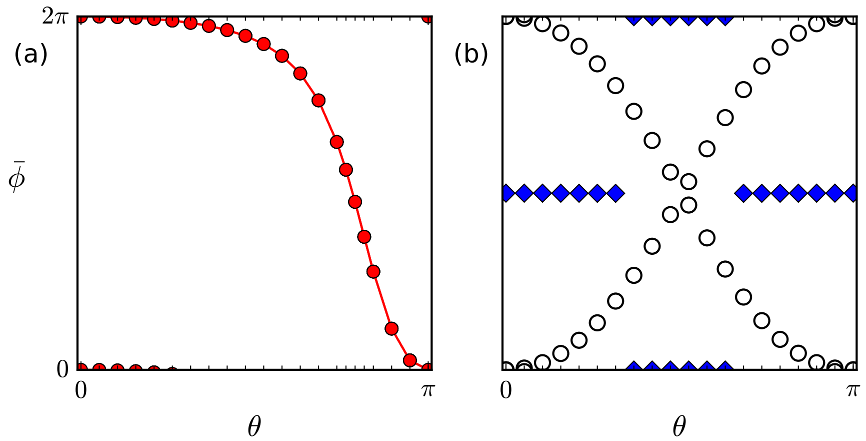


Figure 6: (a) Chern number calculation on a sphere enclosing a single Weyl point with chiral charge -1. (b) Wannier charge centers on a sphere enclosing all four Weyl points.

number calculation for a single Weyl point. Details on the calculation (and the definitions of the labels $\phi$ and $\theta$ in Fig. 6(a)) can be found in the supplementary information of Ref. [16].

In Fig. 6(b) the sphere contains all four Weyl points. We set the Fermi level such that two Weyl points contribute to the topological charge, corresponding to the leftmost and rightmost Weyl points in Fig. 3(b) of the main text. Since there are two occupied states two hybrid Wannier centers are shown (open circles) in Fig. 6(b). The crossing of the two hybrid Wannier centers is analogous to a $Z_2$ invariant of Kane-Mel [13], which is non-trivial in the case shown. This classification can also be used with mirror symmetry and allow for a classification of the triple crossing points. However, both triple crossing points need to be contained in the sphere, otherwise the occupied and unoccupied states are not separated by an energy gap.

# 5 Landé $g$-factor

In the main text we propose gate-defined wires in thin films of $InAs_{0.5}Sb_{0.5}$. Here we estimate the Landé $g$-factor that can be achieved in such a setup.

We first construct effective tight-binding Hamiltonians generated from first-principles Wannier functions [17], using the $s$ and $p$-like orbitals of In and the $p$-like orbitals As and Sb. The Wannier functions are generated without taking spin-orbit interaction into account, which is added afterwards locally to all $p$-orbitals [18]. The atomic spin-orbit interaction constants of In, As and Sb were taken from Ref. [18]. We used these tight-binding models then to calculate the band structure of slabs in various directions with various thicknesses. An in-plane magnetic field is added to the tight-binding Hamiltonian using the scheme of Ref. [19]. Due to the orientation of the magnetic field we can choose the electromagnetic gauge such that the vector potential only changes in the direction orthogonal to the slab, thus not breaking the periodicity of the slab.

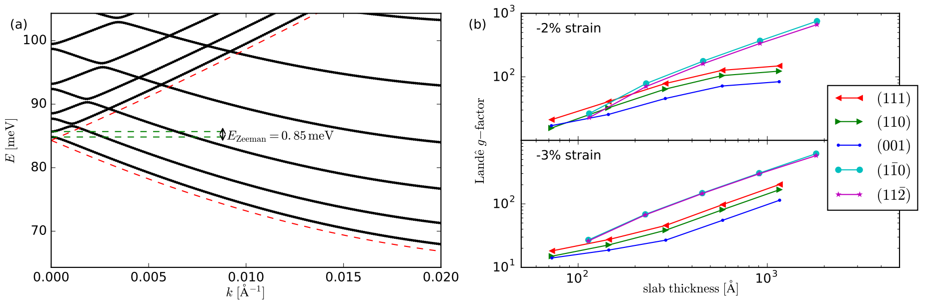


Figure 7: (a) Band structure of a (111)-slab of $InAs_{0.5}Sb_{0.5}$, with 458 Å thickness, -3% (111) strain and an in-plane magnetic field of 0.1 Tesla in (1$\bar{1}$0) direction and $k$ plotted in the same direction. The red dashed lines are the bulk band structure without the magnetic field. (g) Landé $g$-factor of $InAs_{0.5}Sb_{0.5}$ as a function of the slab thickness for the magnetic field in different directions and different strain levels.

In Fig. 7(a) we show the typical band structure of a (111)-slab of $InAs_{0.5}Sb_{0.5}$ at a magnetic field of 0.1 Tesla. The Landé $g$-factor is extracted from the Zeeman splitting $E_{\mathrm{Zeeman}} = \mu_B\, g\, B$ of the subband energetically closest to the first bulk conduction band at $\Gamma$. For magnetic field in the (111), (110) and (001) direction we use (1$\bar{1}$0)-slabs and for the magnetic field in (1$\bar{1}$0) and (11$\bar{2}$) we use (111)-slabs. The $g$-factor is evaluated in a magnetic field of $B = 0.001$ Tesla, ensuring that the Zeeman gap is smaller than the subband gap for all considered slab sizes. The resulting $g$-factors as a function of the slab thickness are plotted in Fig. 7(b). The values of the $g$-factor at 500 Å thickness were obtained via interpolating between adjacent calculated slab thicknesses.

# References

[1] G. Kresse and J. Furthmüller, “Efficient iterative schemes for *ab initio* total-energy calculations using a plane-wave basis set,” *Phys. Rev. B*, vol. 54, pp. 11169–11186, Oct 1996.

[2] G. Kresse and J. Furthmüller, “Efficiency of ab-initio total energy calculations for metals and semiconductors using a plane-wave basis set,” *Computational Materials Science*, vol. 6, no. 1, pp. 15 – 50, 1996.

[3] G. Giesecke and H. Pfister, “Präzisionsbestimmung der Gitterkonstanten von $A_{III}B_V$-Verbindungen,” *Acta Crystallographica*, vol. 11, pp. 369–371, May 1958.

[4] J. P. Perdew, K. Burke, and M. Ernzerhof, “Generalized gradient approximation made simple,” *Phys. Rev. Lett.*, vol. 77, pp. 3865–3868, Oct 1996.

[5] J. Heyd, G. E. Scuseria, and M. Ernzerhof, “Hybrid functionals based on a screened Coulomb potential,” *The Journal of Chemical Physics*, vol. 118, no. 18, pp. 8207–8215, 2003.

[6] J. Heyd and G. E. Scuseria, "Efficient hybrid density functional calculations in solids: Assessment of the Heyd–Scuseria–Ernzerhof screened Coulomb hybrid functional," *The Journal of Chemical Physics*, vol. 121, no. 3, pp. 1187–1192, 2004.

[7] J. Heyd, G. E. Scuseria, and M. Ernzerhof, "Erratum: "Hybrid functionals based on a screened Coulomb potential" [j. chem. phys.118, 8207 (2003)]," *The Journal of Chemical Physics*, vol. 124, no. 21, p. 219906, 2006.

[8] G. B. Stringfellow and G. S. Chen, "Atomic ordering in III/V semiconductor alloys," *Journal of Vacuum Science & Technology B*, vol. 9, no. 4, pp. 2182–2188, 1991.

[9] J. C. Slater and G. F. Koster, "Simplified LCAO method for the periodic potential problem," *Phys. Rev.*, vol. 94, pp. 1498–1524, Jun 1954.

[10] P. Sengupta, H. Ryu, S. Lee, and Y. Tan, "Numerical guidelines for setting up a general purpose k.p simulator with applications to quantum dot heterostructures and topological insulators," *ArXiv e-prints*, Sept. 2014.

[11] S. Jeon, B. B. Zhou, A. Gyenis, B. E. Feldman, I. Kimchi, A. C. Potter, Q. D. Gibson, R. J. Cava, A. Vishwanath, and A. Yazdani, "Landau quantization and quasiparticle interference in the three-dimensional Dirac semimetal $Cd_3As_2$," *Nat Mater*, vol. 13, pp. 851–856, 09 2014.

[12] D. J. Thouless, M. Kohmoto, M. P. Nightingale, and M. den Nijs, "Quantized Hall conductance in a two-dimensional periodic potential," *Phys. Rev. Lett.*, vol. 49, pp. 405–408, Aug 1982.

[13] C. L. Kane and E. J. Mele, "$Z_2$ topological order and the Quantum Spin Hall effect," *Phys. Rev. Lett.*, vol. 95, p. 146802, Sep 2005.

[14] A. A. Soluyanov and D. Vanderbilt, "Computing topological invariants without inversion symmetry," *Phys. Rev. B*, vol. 83, p. 235401, Jun 2011.

[15] D. Gresch, M. Troyer, A. Soluyanov, G. Autes, O. Yazyev, A. Bernevig, and D. Vanderbilt, "Universal framework for identifying topological materials and its numerical implementation in z2pack software package," in *APS Meeting Abstracts*, 2016.

[16] A. A. Soluyanov, D. Gresch, Z. Wang, Q. Wu, M. Troyer, X. Dai, and B. A. Bernevig, "Type-II Weyl semimetals," *Nature*, vol. 527, p. 495, Nov. 2015.

[17] A. A. Mostofi, J. R. Yates, Y.-S. Lee, I. Souza, D. Vanderbilt, and N. Marzari, "wannier90: A tool for obtaining maximally-localised Wannier functions," *Computer physics communications*, vol. 178, no. 9, pp. 685–699, 2008.

[18] D. J. Chadi, "Spin-orbit splitting in crystalline and compositionally disordered semiconductors," *Phys. Rev. B*, vol. 16, pp. 790–796, Jul 1977.

[19] M. Graf and P. Vogl, "Electromagnetic fields and dielectric response in empirical tight-binding theory," *Phys. Rev. B*, vol. 51, pp. 4940–4949, Feb 1995.
